# Supplementary material for: Numerical simulation, clustering and prediction of multi-component polymer precipitation
Source: arXiv:2007.07276 ancillary file (2020-08-26)
Supplement: Supplementary file 1 [file supplementary.pdf]

# 1 Autoencoder Hyperparameters

## 1.1 Dense autoencoders

The following list documents the hyperparameters explored during the hyperparameters optimisation step for the Dense autoencoders.

1. The activation function. This is the function that determines the output of a neuron in the neural network. The following activation functions are tested: 1) Rectified Linear Unit (ReLU), 2) Exponential Linear Unit (ELU) and 3) Sigmoid. The activation function for the last layer was kept as ‘Sigmoid’
2. The loss function. This is the error function which is evaluated during the neural network training stage and the training strives to minimise the losses. The following loss functions were tested: ‘logcosh’, ‘mean\_squared\_error’, ‘binary\_crossentropy’ and ‘poisson’.
3. The optimizer. This is the optimization algorithm that is used to minimize the loss. The following optimizers were tested: ‘Adam’, ‘adam’, ‘RMSprop’.
4. The number of nodes in the hidden layers. If the architecture has hidden layers, the following values were tested : 2048, 1024, 512, 256 and 128.
5. Dropout. Dropout causes a fraction of neurons to be discarded randomly during training. This helps to reduce overfitting. Values of dropout tested are 0, 0.1 and 0.2.
6. Shuffling. This option shuffles the data during the training phase before each epoch. This helps reduce overfitting of the neural network. This is a boolean parameter with either ‘true’ or ‘false’.
7. Batch Size. The batch size is the number of samples per gradient update. The following values were tested: 100, 200, 300 and 629. For the larger neural networks, e.g. Dense-3, the batch size was clipped to between 100 and 200 due to memory constraints.
8. The number of hidden layers in the encoder and decoder sections. The architecture of an autoencoder is typically symmetric, hence the number of layers and nodes per layer in the encoder and decoder are the same. 0, 1 and 2 hidden layers in the encoder/decoder section are tested. This results in the autoencoder having 3, 5 or 7 layers including the input and output.
9. Encoding dimensions. This refers to the number of nodes at the bottleneck and is the dimensionality of the encoded representation of the data. This parameter is first tested within the hyperparameter optimisation with values of 20, 50 and 100 and is further evaluated after an optimal autoencoder structure is selected.
10. Epochs. An epoch is an iteration over the data provided. For the hyperparameter optimization process, this was kept at a low value of 10 for all parameter combinations as the computational time would otherwise become intractable. For Dense 1/2/3 autoencoders, 30 epochs were adequate for convergence.

## 1.2 Convolutional autoencoders

The convolutional autoencoder has similar hyperparameters as the dense autoencoder along with a few more to consider:

1. Number of convolutional layers present. 1 to 3 layers are explored. This also corresponds to the number of MaxPooling layers present as MaxPooling is used to perform spatial down-sampling after each convolutional layer in the encoder section.
2. Number of filters per convolutional layer.
3. Size of the convolutional kernel. This is typically given in the form  $(m,n)$  and typically ranges from  $2\times 2$  to  $10\times 10$  pixels.
4. Size of the MaxPooling pool size which corresponds to the integer factor used to perform downsampling. This was kept at 2.

From the hyperparameter optimisation, for the Dense autoencoders, the following settings were used: activation function = ‘ReLU’, batch size = 100, dropout = 0, loss function = ‘logcosh’, optimiser = ‘Adam’ and shuffling = ‘False’. These results were consistent across the Dense-1 and Dense-2 autoencoders. The optimal Dense-3 autoencoder had the following different settings: activation function = ‘ELU’, loss function = ‘mean\_squared\_error’, optimiser=‘Nadam’ and number of hidden-layer nodes = 128.

Minimal manual hyperparameter optimisation was necessary for Conv autoencoders as the default hyperparameters such as the size of the convolutional kernel ( $3\times 3$ ) and pool size (2) were able to yield satisfactory performance. The batch size was however reduced to 50 due to memory constraints. Hence, these variables were kept constant for Conv and Conv/Dense autoencoders. The deeper the autoencoder, the greater the number of epochs of training were necessary; Conv-3 autoencoders required 75 epochs, Conv-4: 120 and Conv-5: 160.

## 2 Model validation

The following images are obtained both from the work of Nauman and He (1994) and our model. This comparison enables the bench-marking and validation of the implemented code. These simulations correspond to a static PPP case with a range of initial values of  $a_0$  and  $b_0$  and varying values of  $\chi_{ij}$ . From a visual inspection of the rest of the plates, there is more than 90% agreement between our model and the work of Nauman and He (1994), indicating that the developed model is accurate.

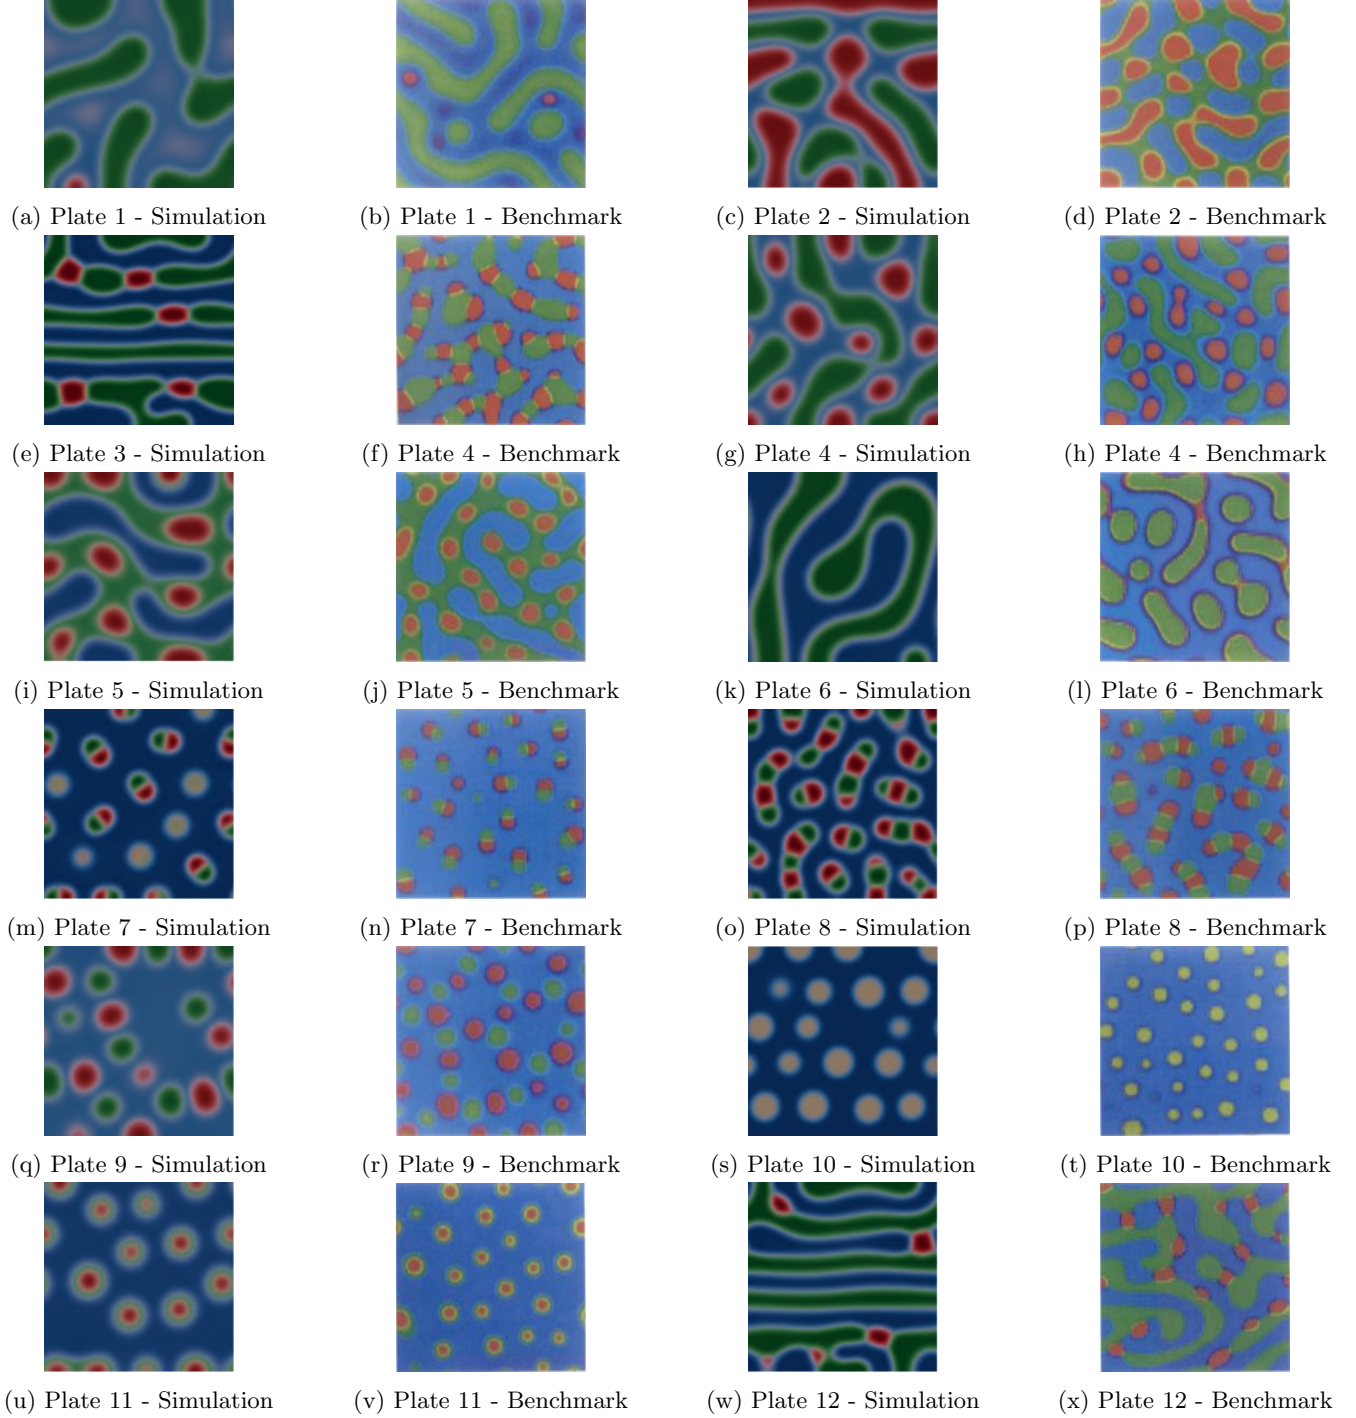

Figure 1: Reproduced simulations (Left) and benchmark results (Right) corresponding to plates 1-12 from Nauman and He Nauman and He (1994).

### 3 Direct manual classification of blend morphology

Table 1: Summary of manual classification with sample images and descriptions

| Cluster number | Morphology description                                                                                                                                                                          | Sample image                                                                        | Cluster number | Morphology description                                                                                                                                                                          | Sample image 2                                                                        |
|----------------|-------------------------------------------------------------------------------------------------------------------------------------------------------------------------------------------------|-------------------------------------------------------------------------------------|----------------|-------------------------------------------------------------------------------------------------------------------------------------------------------------------------------------------------|---------------------------------------------------------------------------------------|
| 0              | Two phases are present, one phase is continuous. The other phase is dispersed as spherical or globular dots.                                                                                    | 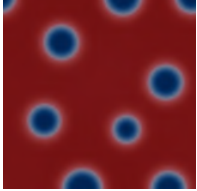   | 1              | Three phases are present, one phase is continuous. The other two phases are dispersed as spherical or globular dots with occasional connectivity between the two phases                         | 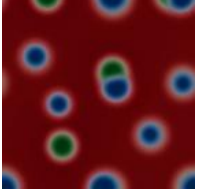   |
| 2              | Three phases are present, one phase is continuous. The other two phases are dispersed as spherical or globular dots.                                                                            | 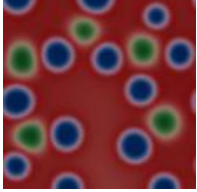   | 3              | Three main phases are present, one phase is continuous. The other two phases form chains of beads with each bead containing one phase.                                                          | 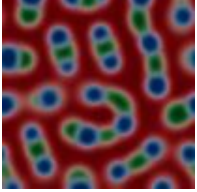   |
| 4              | Three phases are present, one phase is continuous but appears as narrow channels in a weblike manner. The other two phases are dispersed as distorted islands.                                  | 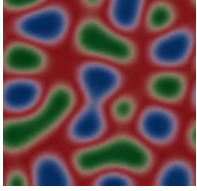   | 5              | Two main phases are present, one phase is continuous. The other phases forms globular or dumbbell shaped islands.                                                                               | 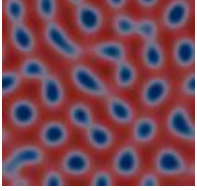   |
| 6              | Three phases are present. None of the phases are continuous and all the phases appear as globular or distorted islands. The islands of each of the phases are of comparable sizes               | 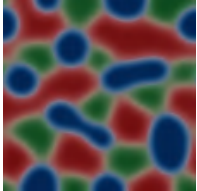  | 7              | Two main phases are present, one phase is continuous with two components present which are well mixed. The other phase forms globular or dumbbell shaped islands.                               | 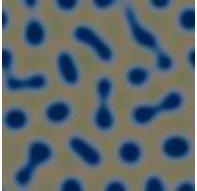  |
| 8              | Three phases are present. Two phases appear in a co-continuous manner with the third phase appearing as globular islands within the channels of one phase.                                      | 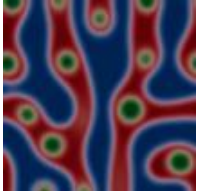 | 9              | Three phases are present. Two phases adopt co-continuous / elongated shapes while the third phase appears as small islands either joining the two larger domains or simply adjoined.            | 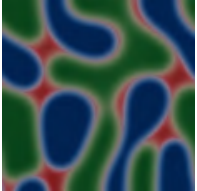 |
| 10             | Three phases are present. One phase is continuous. The other two phases adopt a core-shell morphology where one phase appears as the core and the other phase encapsulates the core as a shell. | 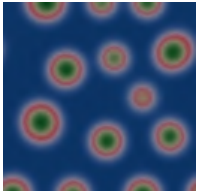 | 11             | Three phases are present. One phase is continuous with the other two phases adopt a Janus particle morphology. Occasionally, globular particles of one or two mixed components will be present. | 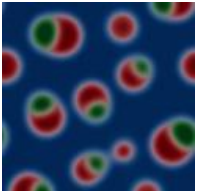 |
| 12             | Two main phases are present. One phase is continuous. The other phase consists of two components which are mixed and appear as globular or dumbbell shaped islands                              | 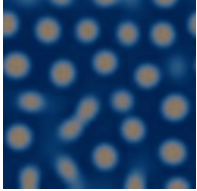 | 13             | Two main phases are present. Both components adopt a co-continuous structure. The third component may accumulate at the interface between the two co-continuous phases.                         | 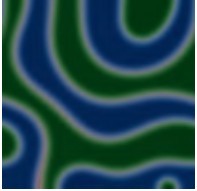 |
| 14             | Two main phases are present. One phase is continuous. The other phase adopts comparatively larger globular and rod-like structures.                                                             | 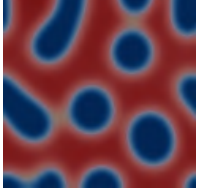 | -              | -                                                                                                                                                                                               | -                                                                                     |

## 4 Manual classification of blend morphology following dimensional reduction with Conv-4 and t-SNE

Table 2: Summary of manual classification with sample images and descriptions

| Cluster number | Morphology description                                                                                                                                                                                    | Sample image                                                                        | Cluster number | Morphology description                                                                                                                                                                                                            | Sample image 2                                                                        |
|----------------|-----------------------------------------------------------------------------------------------------------------------------------------------------------------------------------------------------------|-------------------------------------------------------------------------------------|----------------|-----------------------------------------------------------------------------------------------------------------------------------------------------------------------------------------------------------------------------------|---------------------------------------------------------------------------------------|
| 0              | 2-3 phases are present, The red phase is continuous. The other phases are dispersed as spherical or globular dots. The dots are comparatively spaced out.                                                 | 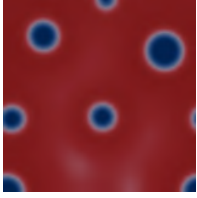   | 1              | 2-3 phases are present, The red phase is continuous. The other phases are dispersed as spherical or globular dots which can be connected in the form of chains and janus particles. The dots are comparatively closer.            | 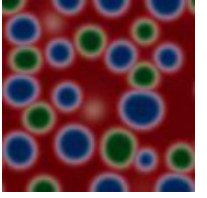   |
| 2              | 2 phases are present, The red phase is continuous. The blue phase is dispersed as spherical or globular dots. The dots are comparatively closer.                                                          | 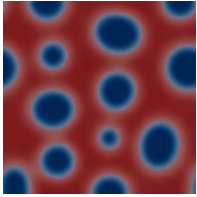   | 3              | 2-3 phases are present, The red phase is mostly continuous, taking on a web-like form. The other phases are dispersed as spherical or globular dots with more frequent connectivity as chains. The dots are comparatively closer. | 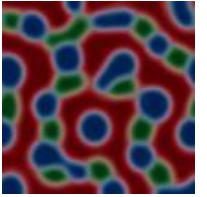   |
| 4              | 2 phases are present, The red phase is continuous. The blue phase is dispersed as larger spherical globs, rods or dumbbells. This cluster is conceptually similar to 2                                    | 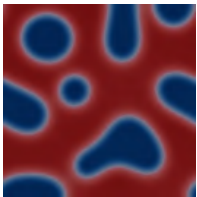  | 5              | 3 phases are present, The red phase appears as either webs or as islands. The other phases are dispersed as islands as well with possibility connectivity as chains.                                                              | 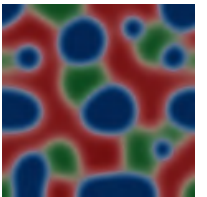  |
| 6              | 3 phases are present, The red phase appears as webs or discrete islands. The blue phase is dispersed as larger spherical globs, rods or dumbbells. This cluster is conceptually similar to 2              | 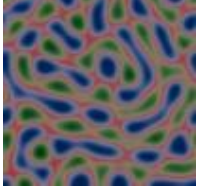 | 7              | 2 phases are present, The red phase is continuous. The blue phase appears as globular dots and/or elongated rods.                                                                                                                 | 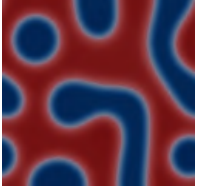 |
| 8              | 3 phases are present. Each of these phases appear as discrete islands with no phase appearing continuously.                                                                                               | 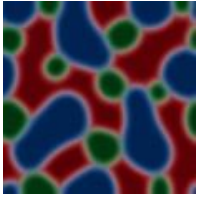 | 9              | 2 phases are present, The blue phase appears as small channels or dumbbells that appear throughout the domain. The other phase appears with a similar pattern, but consist of the red and green phases mixing together.           | 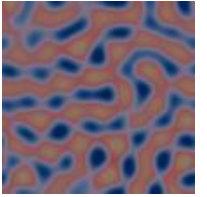 |
| 10             | 3 phases are present. Each of these phases appear as discrete islands with no phase appearing continuously. This is similar to cluster 8.                                                                 | 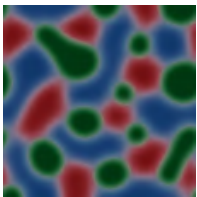 | 11             | 3 phases are present. The red phase appears as thin webs and the green and blue phases appear as thin rods and globular structures. There is overlap with cluster 6.                                                              | 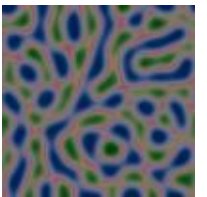 |
| 12             | 3 phases are present. The blue and green phases appear co-continuously with the red phase appearing as discrete islands adjoined to the green phase or forming a layer between the green and blue phases. | 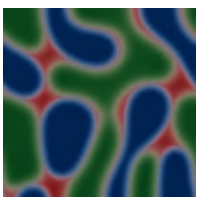 | 13             | 2 phases are present. Blue and green phases appears as co-continuous phases.                                                                                                                                                      | 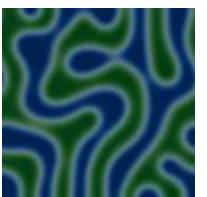 |

| Cluster number | Morphology description                                                                                                                                   | Sample image                                                                       | Cluster number | Morphology description                                                                                                                                                  | Sample image 2                                                                       |
|----------------|----------------------------------------------------------------------------------------------------------------------------------------------------------|------------------------------------------------------------------------------------|----------------|-------------------------------------------------------------------------------------------------------------------------------------------------------------------------|--------------------------------------------------------------------------------------|
| 14             | 2 phases are present. The red and blue phases appear as co-continuous phases.                                                                            | 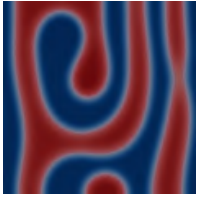  | 15             | 3 phases are present. Blue and red phases appear as co-continuous phases. The green phase appears as globular islands in the form of chains or within the red channels. | 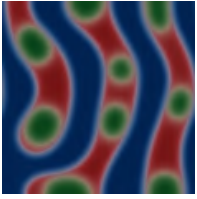  |
| 16             | Identical to cluster 9.                                                                                                                                  | 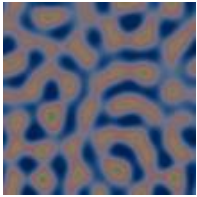  | 17             | This cluster is conceptually identical to cluster 15, but the red and green phases are reversed.                                                                        | 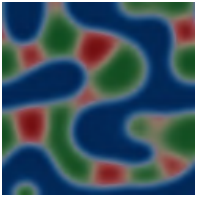  |
| 18             | Identical to cluster 13.                                                                                                                                 | 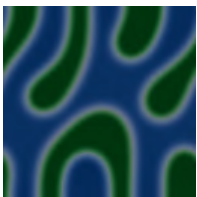  | 19             | This cluster is conceptually identical to cluster 4, but the blue and red phases are reversed.                                                                          | 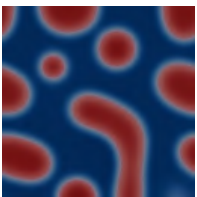  |
| 20             | Three phases are present. The blue phase is continuous and the red and green phases adopted a core-shell morphology with the green phase being the core. | 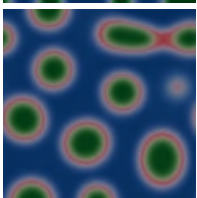  | 21             | This cluster is conceptually identical to cluster 19, but the red phase is replaced with green.                                                                         | 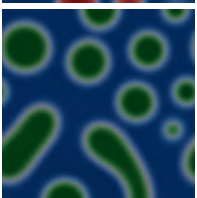  |
| 22             | Similar to cluster 20. However, the size of the core-shell structures are smaller                                                                        | 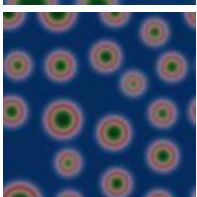 | 23             | This cluster is conceptually identical to cluster 2, but the red phase is replaced with blue and the blue phase is replaced with green.                                 | 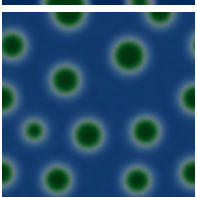 |

## 5 Affinity propagation clustering of blend morphology following dimensional reduction with Conv-4 and t-SNE

Table 3: Summary of manual classification with sample images and descriptions

| Cluster number | Morphology description                                                                                                                                                                                         | Sample image                                                                        | Cluster number | Morphology description                                                                                                                                                                                                                                                              | Sample image 2                                                                        |
|----------------|----------------------------------------------------------------------------------------------------------------------------------------------------------------------------------------------------------------|-------------------------------------------------------------------------------------|----------------|-------------------------------------------------------------------------------------------------------------------------------------------------------------------------------------------------------------------------------------------------------------------------------------|---------------------------------------------------------------------------------------|
| 0              | 2-3 phases are present, The red phase is continuous. The other phases are dispersed as spherical or globular dots. The dots are comparatively spaced out.                                                      | 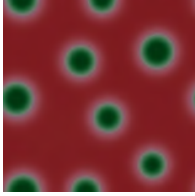   | 1              | 2-3 phases are present, The red phase is continuous. The other phases are dispersed as spherical or globular dots which can be connected in the form of chains and janus particles. The dots are comparatively closer.                                                              | 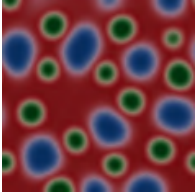   |
| 2              | 3 phases are present. The red phase is continuous, forming web-like channels of varying thickness. The other phases are dispersed as spherical or globular dots which frequently are connected to form chains. | 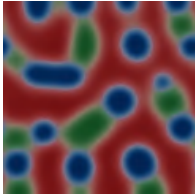   | 3              | 2 phases are present. The red phase is continuous. The blue phase appears as spherical particles or rods / dumbbells.                                                                                                                                                               | 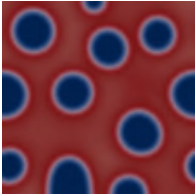   |
| 4              | 3 phases are present. The red phase is continuous, forming web-like channels of varying thickness. The other phases are dispersed as spherical or globular dots which frequently are connected to form chains. | 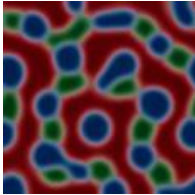  | 5              | 3 phases are present. None of the phases are continuous with each phase forming islands that are in contact with the other phases.                                                                                                                                                  | 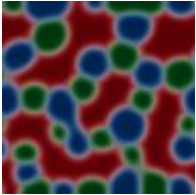  |
| 6              | Similar to cluster 3.                                                                                                                                                                                          | 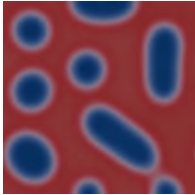 | 7              | 3 phases are present. The red phase is continuous with a web-like morphology of varying thickness. The blue phase appears as channels or distorted islands and the green phase appears as islands. Occasional connectivity between green and blue phases to form chains is present. | 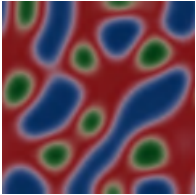 |
| 8              | Similar to cluster 7.                                                                                                                                                                                          | 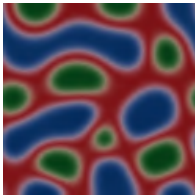 | 9              | Similar to cluster 5. The islands formed by the green and blue phases are comparatively larger.                                                                                                                                                                                     | 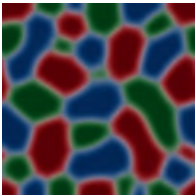 |
| 10             | Similar to cluster 9.                                                                                                                                                                                          | 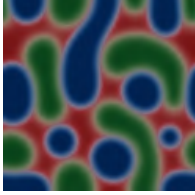 | 11             | Similar to cluster 6. However the blue phase forms longer rods and distorted globular structures.                                                                                                                                                                                   | 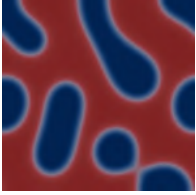 |
| 12             | Similar to cluster 9.                                                                                                                                                                                          | 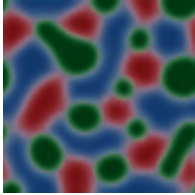 | 13             | 3 phases are present. The blue and green phases form channels with the red phase accumulating as discrete islands connecting the channels or at the interface between the blue and green phase.                                                                                     | 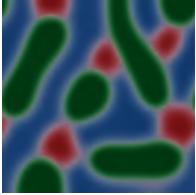 |

| Cluster number | Morphology description                                                                                                                          | Sample image                                                                      | Cluster number | Morphology description                                                          | Sample image 2                                                                      |
|----------------|-------------------------------------------------------------------------------------------------------------------------------------------------|-----------------------------------------------------------------------------------|----------------|---------------------------------------------------------------------------------|-------------------------------------------------------------------------------------|
| 14             | 2 phases are present. The blue and green phases adopt a co-continuous morphology.                                                               | 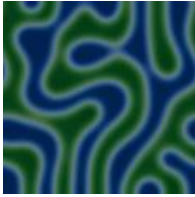 | 15             | 2 phases are present. The blue and red phases adopt a co-continuous morphology. | 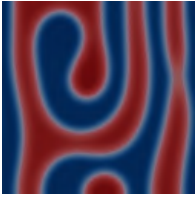 |
| 16             | 3 phases are present. The blue phase is continuous. The red and green phases adopt a chain-like morphology.                                     | 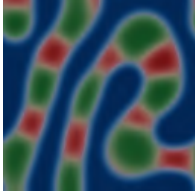 | 17             | Similar to cluster 14.                                                          | 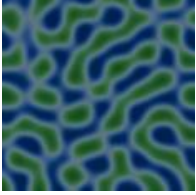 |
| 18             | 2 phases are present. The blue phase is continuous. The red phase adopt a globular dot or rod-like morphology.                                  | 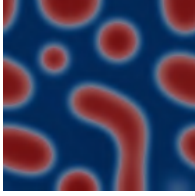 | 19             | Similar to cluster 18. But the red phase is replaced by green.                  | 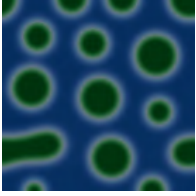 |
| 20             | 3 phases are present. The blue phase is continuous. The red and green phases adopt a core-shell morphology with the green phase being the core. | 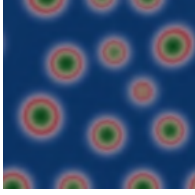 |                |                                                                                 |                                                                                     |

## 6 Convolutional autoencoder image reconstruction

The dimensionality of the embedding can be understood as a product of the number of convolutional layers as captured in the autoencoder structure label and the number of filters at the bottleneck. A Conv-3 autoencoder has the image downsampled by  $2^3 = 8\times$  which results in the dimensionality of each filter being  $25 \times 25 = 625$ . If the bottleneck layer has 3 filters for example, then the dimensionality of the embedding is given by  $625 \times 3 = 1875$ .

Table 4: Reconstructed images from convolutional autoencoders

| Autoencoder structure | 1 Filter<br>(Loss)<br>(Accuracy)                                                    | 2 Filters<br>(Loss)<br>(Accuracy)                                                   | 3 Filters<br>(Loss)<br>(Accuracy)                                                   | 4 Filters<br>(Loss)<br>(Accuracy)                                                     | 5 Filters<br>(Loss)<br>(Accuracy)                                                     |
|-----------------------|-------------------------------------------------------------------------------------|-------------------------------------------------------------------------------------|-------------------------------------------------------------------------------------|---------------------------------------------------------------------------------------|---------------------------------------------------------------------------------------|
| Conv-3                | 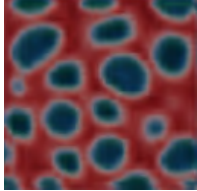   | 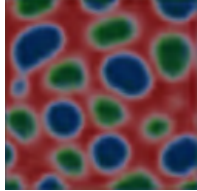   | 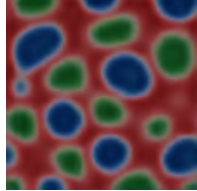   | 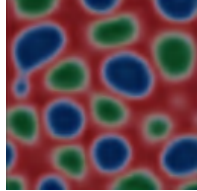   | -                                                                                     |
|                       | 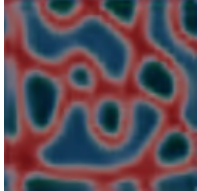   | 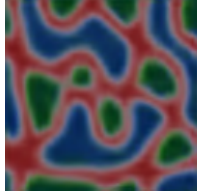   | 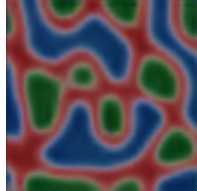   | 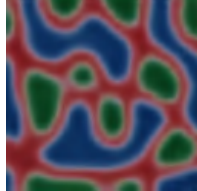   |                                                                                       |
|                       | (0.0020)<br>(0.8171)                                                                | $(9.6092 \times 10^{-4})$<br>(0.9312)                                               | $(5.2737 \times 10^{-4})$<br>(0.9614)                                               | $(4.5042 \times 10^{-4})$<br>(0.9654)                                                 |                                                                                       |
| Conv-4                | 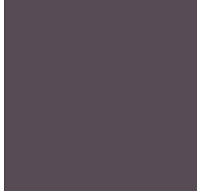  | 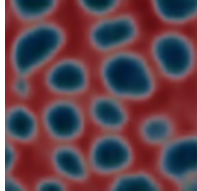  | 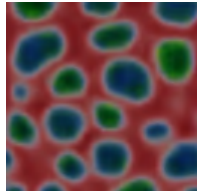  | 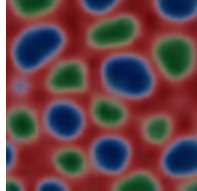  | -                                                                                     |
|                       | 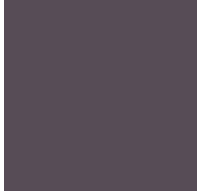 | 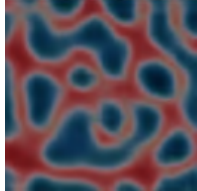 | 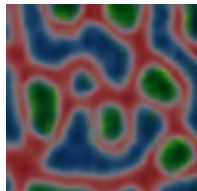 | 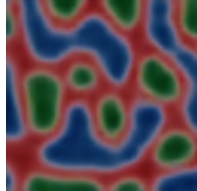 |                                                                                       |
|                       | (0.0121)<br>(0.4318)                                                                | (0.0027)<br>(0.8016)                                                                | (0.0018) // (0.8617)                                                                | (0.0012)<br>(0.9280)                                                                  |                                                                                       |
| Conv-5                | 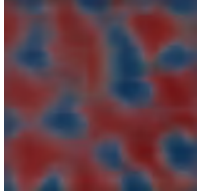 | 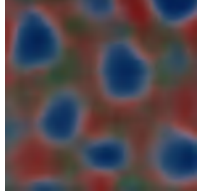 | 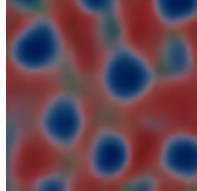 | 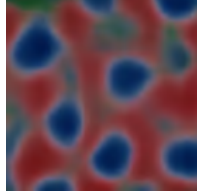 | 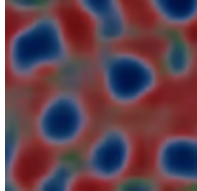 |
|                       | 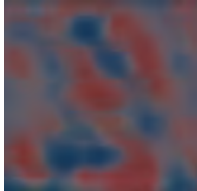 | 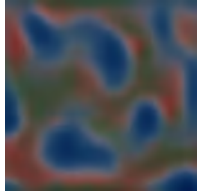 | 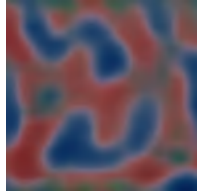 | 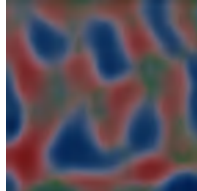 | 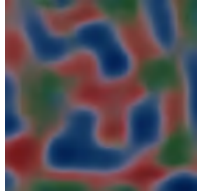 |
|                       | (0.0079)<br>(0.6804)                                                                | (0.0060)<br>(0.7516)                                                                | (0.0051)<br>(0.7905)                                                                | (0.0050)<br>(0.7949)                                                                  | (0.0042)<br>(0.8225)                                                                  |

## References

Nauman, E. B. and He, D. Q. (1994). Morphology predictions for ternary polymer blends undergoing spinodal decomposition. *Polymer*, 35(11):2243–2255.
